# Supplementary material for: How Low Can You Go? Searching for the Intrinsic Dimensionality of Complex Networks using Metric Node Embeddings
Source: arXiv:2503.01723 source file (2025-03-03)
Supplement: Supplementary file 1 [file supplementary.tex]

\section{Supplementary}

\subsection{Generalization of the loss function}
The formulation formulation motivates other potential loss functions.

\subsubsection{Hinge loss}
We define the hinge loss in our context as
$\mathcal{L}_H(\mathcal{R}) \mathdef \sum_{i,j} \max(0, 1 - \tilde{a}_{i,j}\mathcal{R}_{i,j})$.
\todo{Write about this}

\subsubsection{Poisson loss} If we model the probability of a link with a Poisson distribution such that ...
\(\mathcal{L}_P\)
\todo{Write about this}

\subsubsection{Generalized objective}

\todo{Proof or intuition that we optimize for the same objective across losses}
